# Supplementary material for: Probing the Top-Higgs Sector with Composite Higgs Models at Present and Future Hadron Colliders
Source: arXiv:2008.13026 ancillary file (2020-08-29)
Supplement: Supplementary file 1 [file cluster_plots.pdf]

# **Ancillary Material to: “Probing the Top-Higgs Sector with Composite Higgs Models at Present and Future Hadron Colliders”**

**Carlos Bautista,<sup>1,2</sup> Leonardo de Lima,<sup>3</sup> Ricardo D’Elia  
Matheus,<sup>1</sup> Eduardo Pontón,<sup>1,2,5</sup> Leônidas A. Fernandes  
do Prado,<sup>1,4</sup> and Aurore Savoy-Navarro<sup>4</sup>**

<sup>1</sup>Instituto de Física Teórica – UNESP, São Paulo, Brazil

<sup>2</sup>ICTP South American Institute for Fundamental Research, São Paulo, Brazil

<sup>3</sup>Universidade Tecnológica Federal do Paraná, Toledo, Brazil

<sup>4</sup>IRFU-CEA, Université Paris-Saclay and CNRS-IN2P3, France

E-mail: [carlos.bautista@unesp.br](mailto:carlos.bautista@unesp.br), [leonardolima@utfpr.edu.br](mailto:leonardolima@utfpr.edu.br),  
[matheus@ift.unesp.br](mailto:matheus@ift.unesp.br), [leonidas.prado@cern.ch](mailto:leonidas.prado@cern.ch), [aurore.savoy.navarro@cern.ch](mailto:aurore.savoy.navarro@cern.ch)

---

<sup>5</sup>Eduardo greatly contributed to the work here presented but sadly passed away in the early stages of the writing of this document. He will be sorely missed.

This document contains the plots relative to the clustering of sections 4.3.2, 5.2.1 and 5.2.2 of the main article, according to the table below.

| Model and Scan                | Section (in the main article) | Figures (in this document)              |
|-------------------------------|-------------------------------|-----------------------------------------|
| MCHM <sub>14</sub> Low Scale  | 4.3.2                         | <a href="#">1</a> and <a href="#">2</a> |
| MCHM <sub>5</sub> High Scale  | 5.2.1                         | <a href="#">3</a> and <a href="#">4</a> |
| MCHM <sub>14</sub> High Scale | 5.2.2                         | <a href="#">5</a> and <a href="#">6</a> |

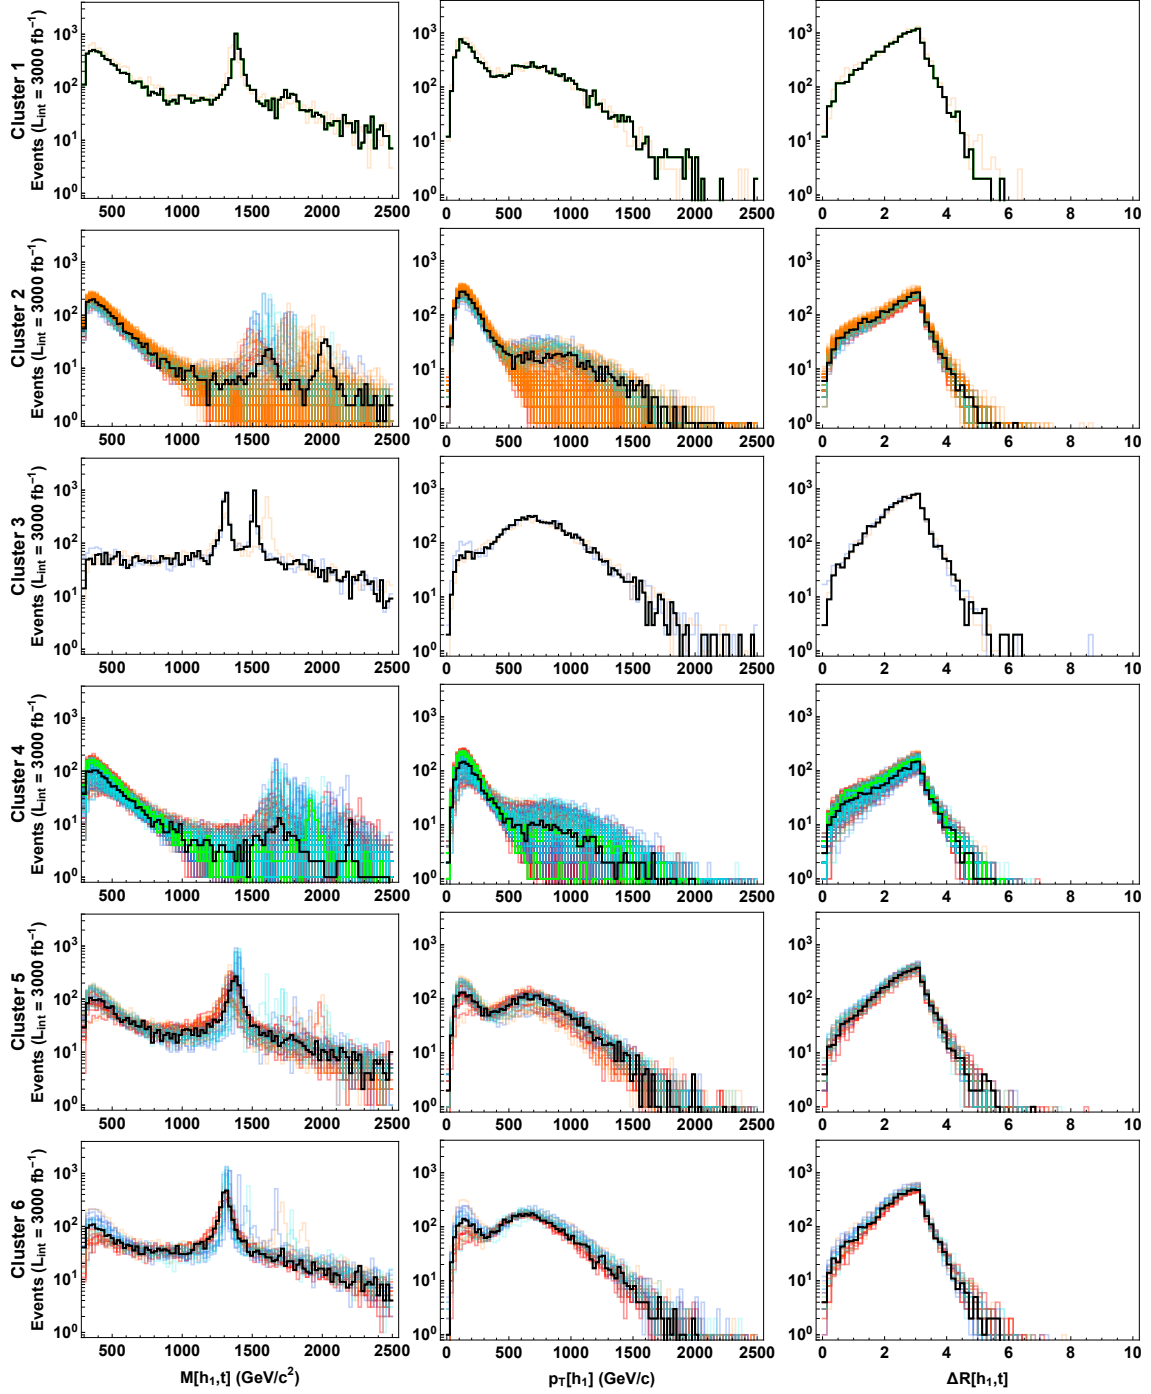

**Figure 1.** Distributions at  $\sqrt{s} = 14$  TeV for the invariant mass of the pair composed by top and most energetic Higgs  $h_1$  (first column), transverse momenta of  $h_1$  (second column) and angular distances in the transverse plane between  $h_1$  and the top (third column), organized in clusters by similarity (clusters 1 through 6). Red, blue, orange and cyan curves indicate respectively points in Regions I, II, III and IV of the MCHM<sub>14</sub>. The benchmark point for each cluster is shown in black, with clusters 1 to 6 containing respectively points  $D_1$  to  $D_6$  in Table 6 of the main article. The example points (Table 2 is the main article) are shown in green (cluster 1 contains  $Q_1$ , cluster 4 contains  $Q_5$  and  $Q_7$ ).

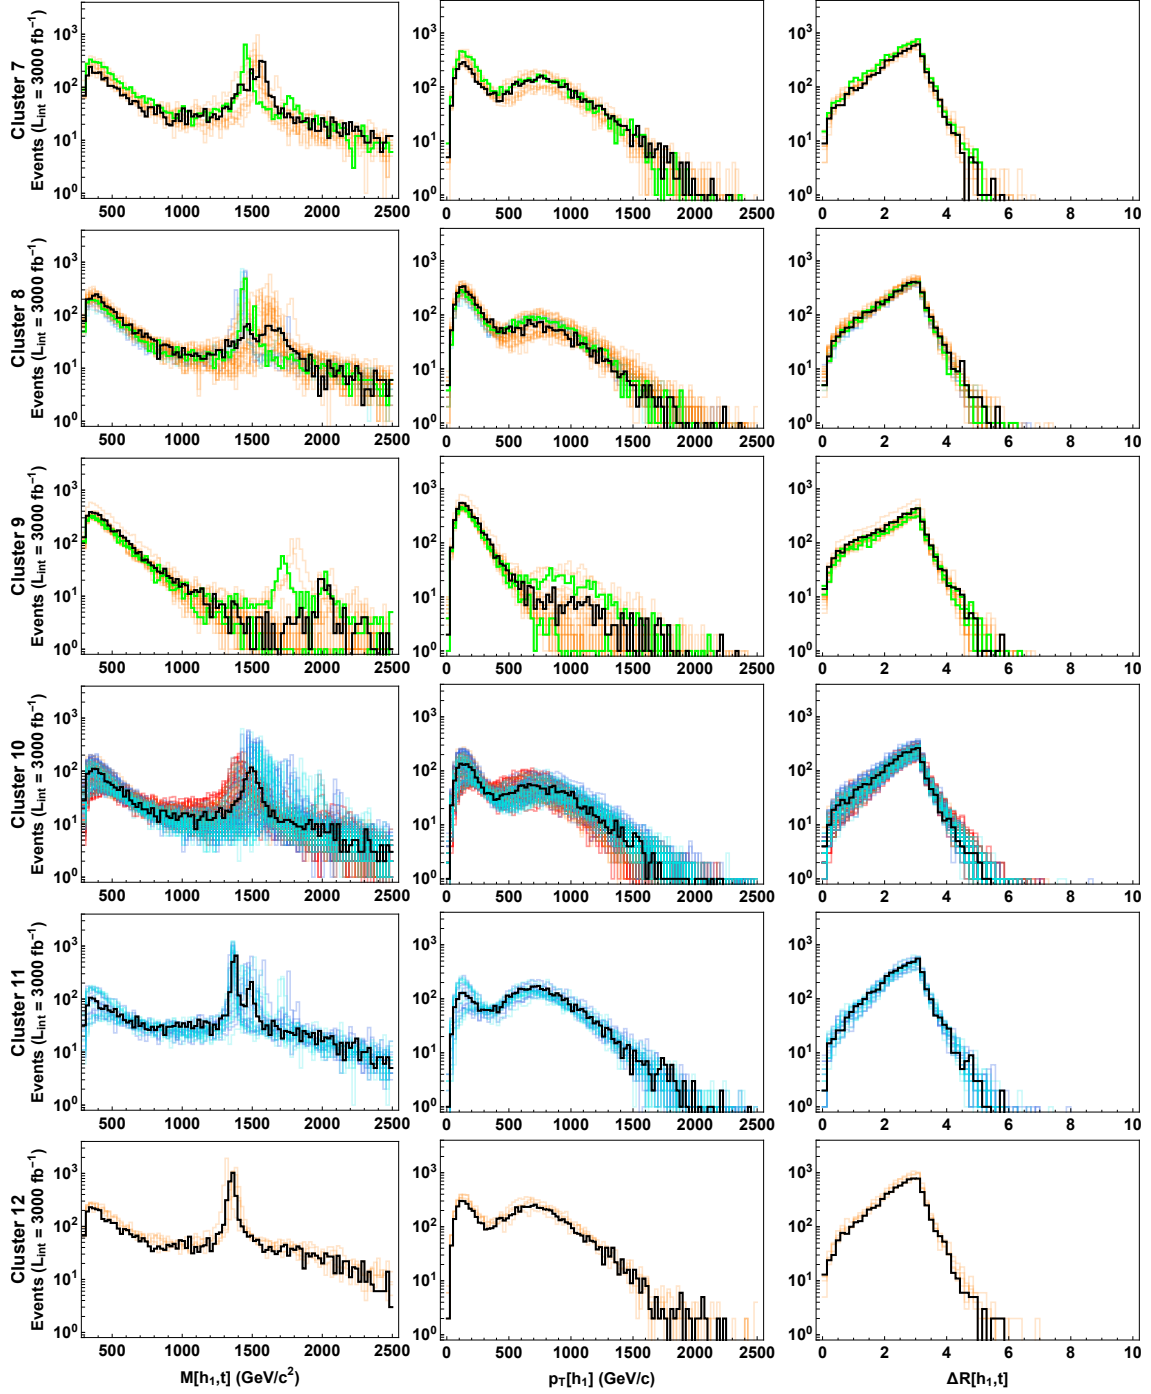

**Figure 2.** Distributions at  $\sqrt{s} = 14$  TeV for the invariant mass of the pair composed by top and most energetic Higgs  $h_1$  (first column), transverse momenta of  $h_1$  (second column) and angular distances in the transverse plane between  $h_1$  and the top (third column), organized in clusters by similarity (clusters 7 through 12). Red, blue, orange and cyan curves indicate respectively points in Regions I, II, III and IV of the MCHM<sub>14</sub>. The benchmark point for each cluster is shown in black, with clusters 7 to 12 containing respectively points  $D_7$  to  $D_{12}$  in Table 6 of the main article. The example points (Table 2 is the main article) are shown in green (cluster 7 contains  $Q_2$ , cluster 8 contains  $Q_6$  and cluster 9 contains  $Q_3$  and  $Q_4$ ).

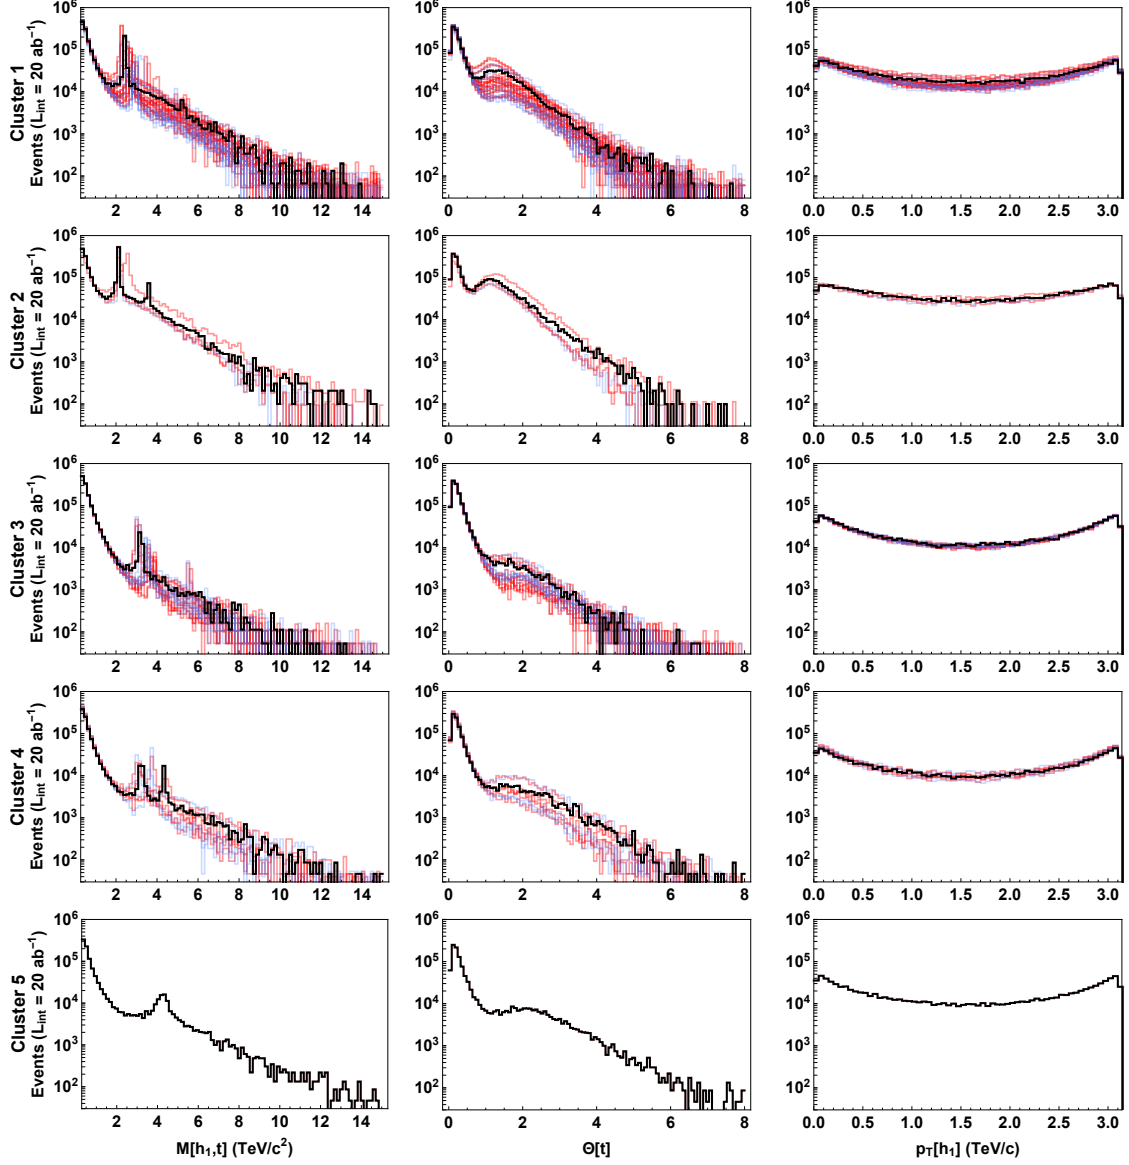

**Figure 3.** Distributions at  $\sqrt{s} = 100$  TeV for the invariant mass of the pair composed by top and most energetic Higgs  $h_1$  (first column), the top quark angle (second column) and the transverse momenta of  $h_1$  (third column), organized in clusters by similarity (clusters 1 through 5). Red and blue curves indicate respectively points in Regions I and II of the MCHM<sub>5</sub>. The benchmark point for each cluster is shown in black, with clusters 1 to 5 containing respectively points  $E_1$  to  $E_5$  in Table 7 of the main article.

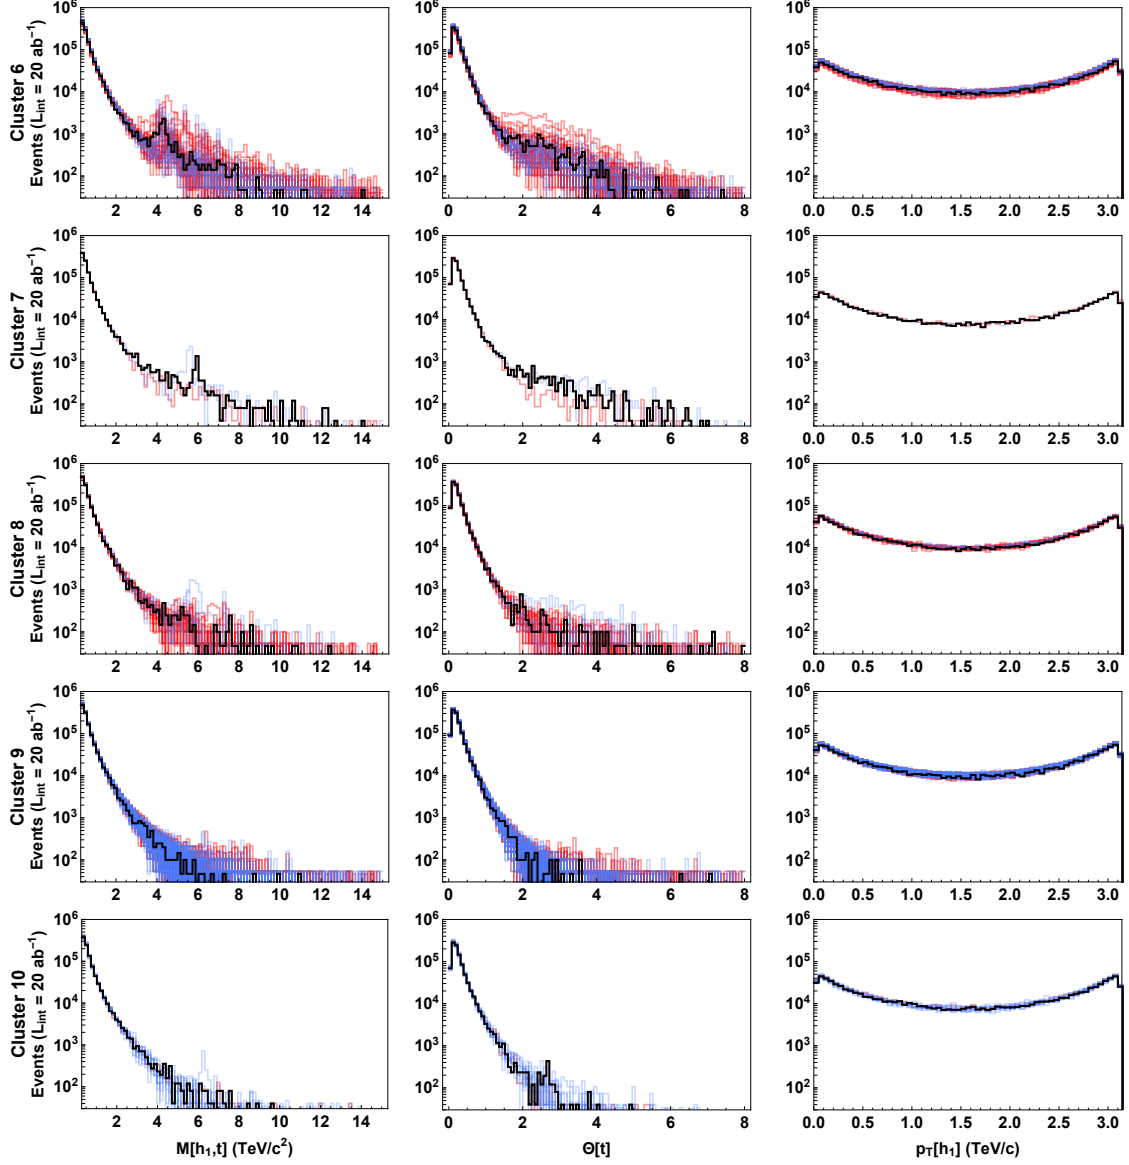

**Figure 4.** Distributions at  $\sqrt{s} = 100$  TeV for the invariant mass of the pair composed by top and most energetic Higgs  $h_1$  (first column), the top quark angle (second column) and the transverse momenta of  $h_1$  (third column), organized in clusters by similarity (clusters 6 through 10). Red and blue curves indicate respectively points in Regions I and II of the MCHM<sub>5</sub>. The benchmark point for each cluster is shown in black, with clusters 6 to 10 containing respectively points  $E_6$  to  $E_{10}$  in Table 7 of the main article.

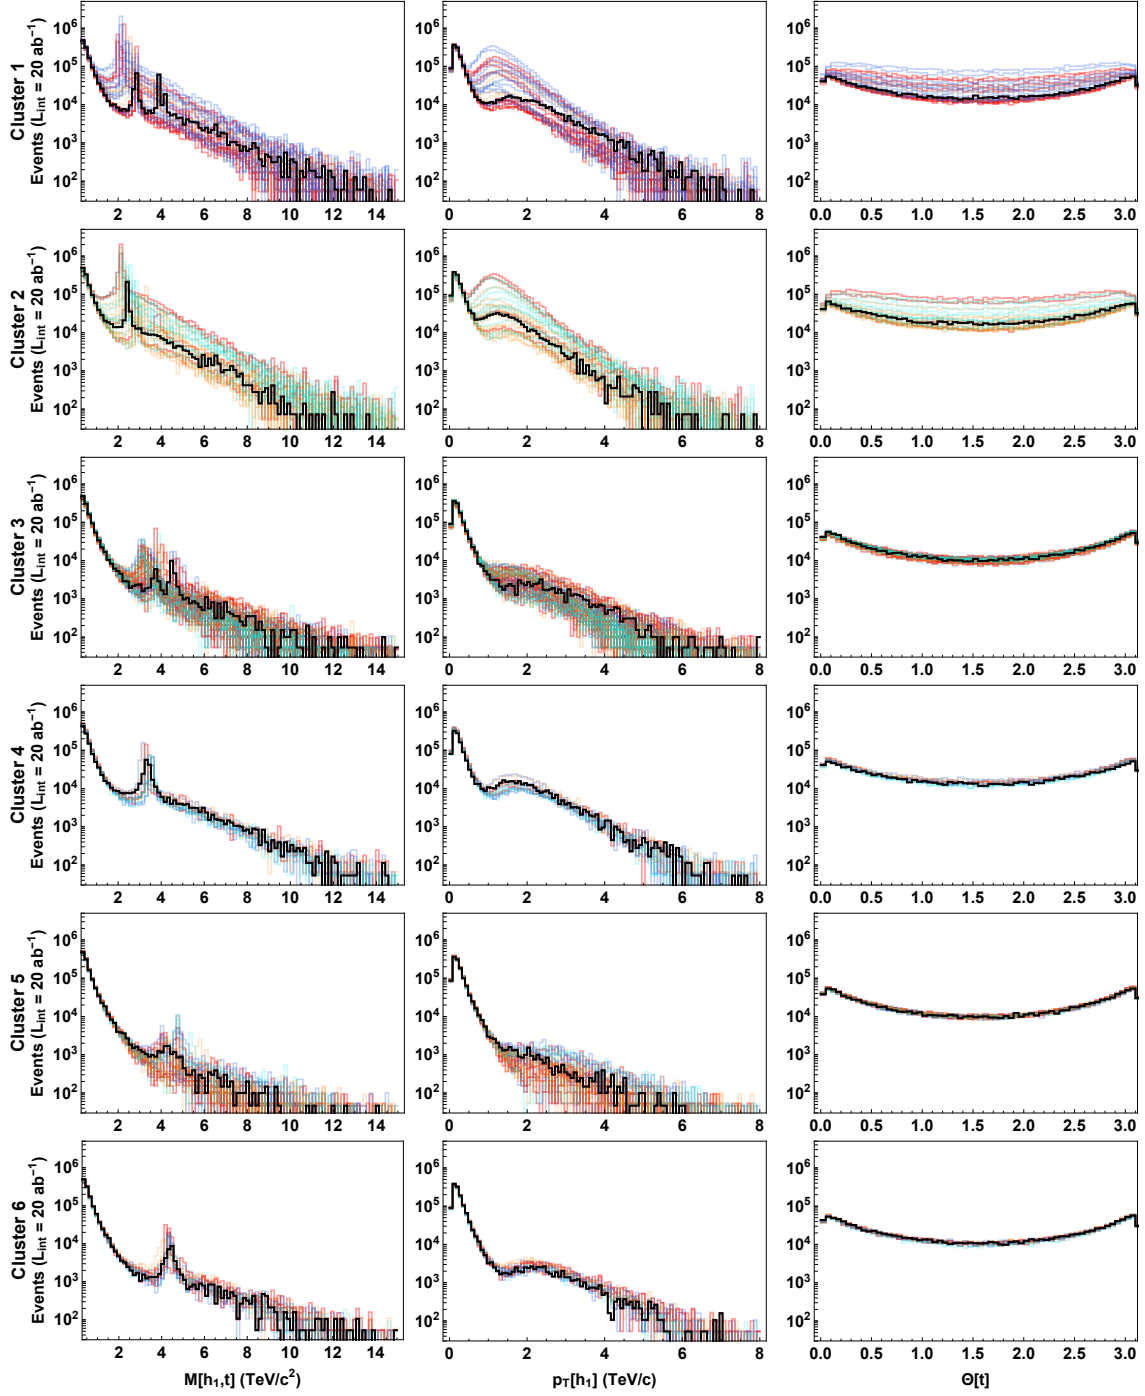

**Figure 5.** Distributions at  $\sqrt{s} = 100$  TeV for the invariant mass of the pair composed by top and most energetic Higgs  $h_1$  (first column), transverse momenta of  $h_1$  (second column) and the top angle (third column), organized in clusters by similarity (clusters 1 through 6). Red, blue, orange and cyan curves indicate respectively points in Regions I, II, III and IV of the MCHM<sub>14</sub>. The benchmark point for each cluster is shown in black, with clusters 1 to 6 containing respectively points  $F_1$  to  $F_6$  in Table 8 of the main article.

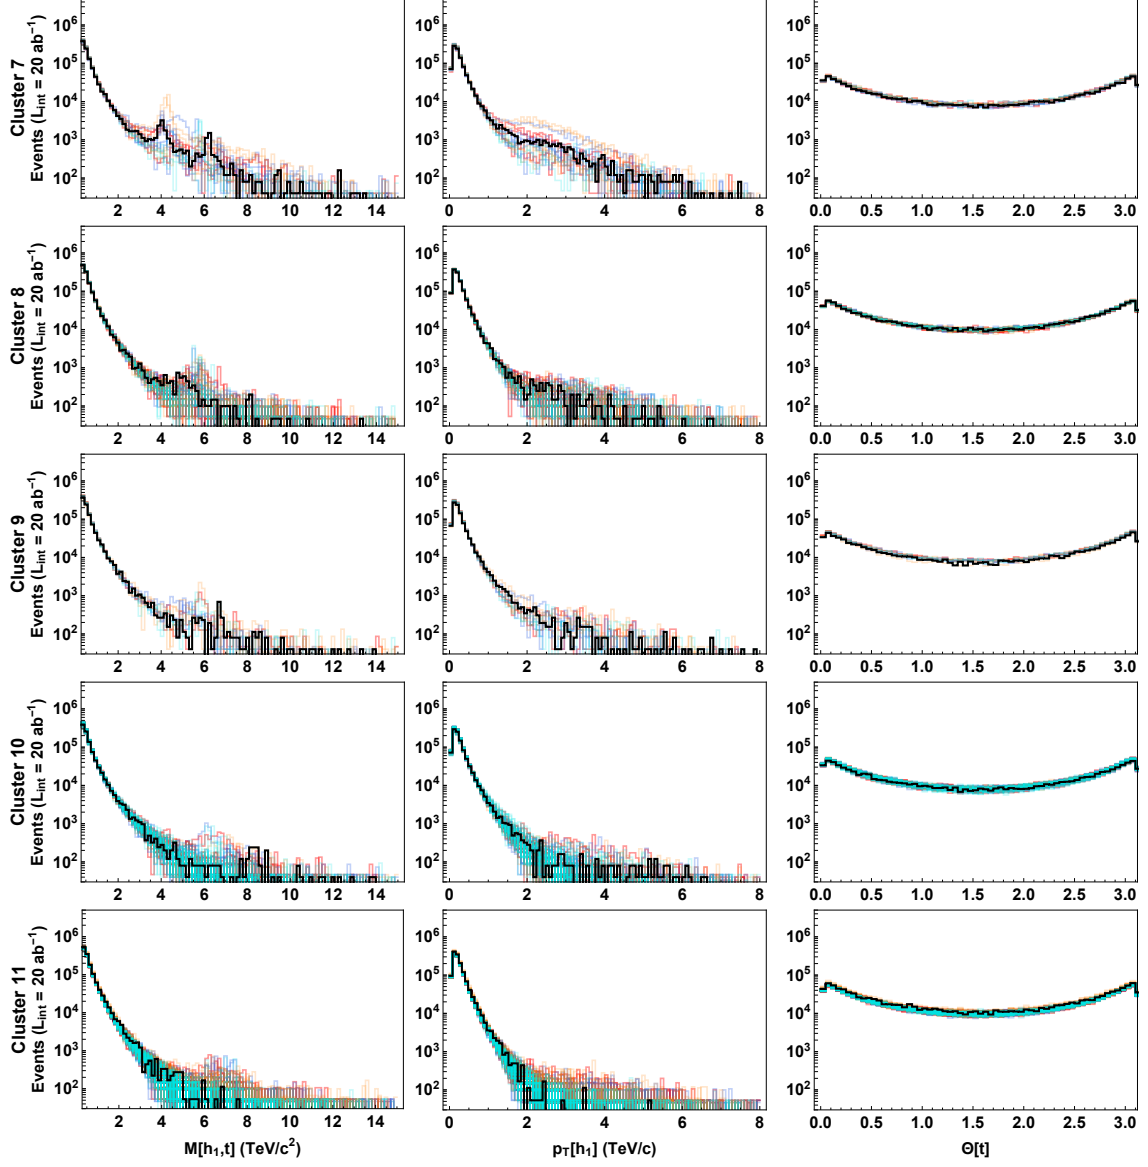

**Figure 6.** Distributions at  $\sqrt{s} = 100$  TeV for the invariant mass of the pair composed by top and most energetic Higgs  $h_1$  (first column), transverse momenta of  $h_1$  (second column) and the top angle (third column), organized in clusters by similarity (clusters 7 through 11). Red, blue, orange and cyan curves indicate respectively points in Regions I, II, III and IV of the  $\text{MCHM}_{14}$ . The benchmark point for each cluster is shown in black, with clusters 1 to 6 containing respectively points  $F_7$  to  $F_{11}$  in Table 8 of the main article.
